# Supplementary material for: Physical Operating-Condition-Guided Vision-Language Matching for Cavitation Diagnosis in Industrial Pipeline Systems
Source: arXiv:2610.27860 source file (2026-10-20)
Supplement: Supplementary file 1 [file appendix.tex]

\section*{Appendix}
\label{sec: Appendix}
\setcounter{table}{0}
\setcounter{figure}{0}
\setcounter{equation}{0}
\setcounter{section}{0}
\setcounter{subsection}{0}
\renewcommand{\thetable}{A\arabic{table}}
\renewcommand{\thefigure}{A\arabic{figure}}
\renewcommand{\theequation}{A.\arabic{equation}}
\renewcommand{\thesection}{A.\arabic{section}}
\renewcommand{\thesubsection}{A.\arabic{subsection}}

\subsection{Definition of Cavitation Intensity}
\label{app: Cavitation Intensity Definition}
Figure \ref{fig: civitation knowledge} illustrates how the local pressure changes in a one-dimensional flow. The valve would operate normally without cavitation when the minimum pressure $p_{\min}$ is higher than the vapor pressure $p_v$. In the case where $p_v>p_{\min}$ cavitation begins. However, it cannot be measured directly as the minimum pressure occurs downstream of the restriction. In practice, the cavitation coefficient $X_{FZ}$ is equal to the ratio of the external pressure difference to the internal pressure difference. It can be determined empirically by assuming that cavitation noise only begins when the minimum pressure $p_{\min}$ is equal to the vapor pressure $p_v$. Therefore, the cavitation coefficient $X_{FZ}$ can be measured by the noise, which depends on the load of the valve. The equations for the cavitation coefficient $X_{FZ}$ and the operating pressure ratio $X_f$ (the pressure recovery factor used in the main text) are given below:
\begin{equation}
X_{FZ}=\frac{p_u-p_d}{p_u-p_{\min}},
\qquad
X_f=\frac{p_u-p_d}{p_u-p_v}.
\end{equation}
where $p_u$ is the upstream pressure, $p_d$ is the downstream pressure, $p_{\min}$ is the minimum pressure in the valve and $p_v$ is the vapor pressure. When all coefficients are known over the full opening range of the valve, the following statements can be made.
\input{input_figs/input_PressureFlowModel.tex}
\begin{itemize}
\item $X_f<X_{FZ}$: The valve operates without cavitation and the flow is only turbulent or laminar.
\item $X_f\geq X_{FZ}$: For $X_f=X_{FZ}$, the valve operates with incipient cavitation. As the difference between $X_{FZ}$ and $X_f$ increases, the cavitation zone grows as the pressure drops due to increasing flow velocities.
\item $X_f>1$: Here the bubbles do not implode in the valve but rather continue to flow into the pipe because the downstream pressure $p_d$ is lower than the vapor pressure $p_v$. This phenomenon is called flashing.
\end{itemize}
The cavitation coefficient $X_{FZ}$ is only applied to the fluid, where it is measured empirically. Its value varies for different liquid mediums, due to changes in viscosity, content of dissolved gas and so on.


\subsection{Acoustic Signal Augmentation}
\label{app: Acoustic Signals Augmentation}
Consistent with the recording index $g$ used in the main text, the original acoustic waveform is represented as $\mathbf{u}_g=[u_{g,1},u_{g,2},\ldots,u_{g,L_g}]^{\mathrm T}\in\mathbb{R}^{L_g\times 1}$, where $L_g$ is the number of samples in recording $g$. The waveform $\mathbf{u}_g$ is distinct from the physical operating-condition vector $\mathbf{x}_g$ associated with the same recording. Given the intentionally maintained steady flow state (i.e., it is always the same flow-state class within each individual measurement lasting \SI{3}{s} or \SI{25}{s}) in each recorded stream and the high temporal resolution of the sensor, each signal can be split into several segments, each containing sufficient information for detection. The segment length is chosen to be sufficiently long to account for the inherent randomness in the noise emission, and each segment can be treated as an independent sample. Therefore, we apply a sliding-window technique $\mathcal{W}(\cdot)$ with window size $W_s$ and step size $S$, as defined in Section \ref{subsec: Datasets and Data Preprocessing}, to obtain $\mathcal{W}(\mathbf{u}_g)=\{\mathbf{u}_{g,n}\}_{n=1}^{N_g}$. Here, $n$ indexes the windows within recording $g$, $\mathbf{u}_{g,n}=[u_{g,(n-1)S+1},\ldots,u_{g,(n-1)S+W_s}]^{\mathrm T}\in\mathbb{R}^{W_s\times 1}$ is the $n$-th subsequence and $N_g=\left\lfloor\frac{L_g-W_s}{S}\right\rfloor+1$ is the number of subsequences. All windows from recording $g$ share the physical operating-condition vector $\mathbf{x}_g$. The sliding-window technique is a crucial part of the acoustic signal preprocessing.

\subsection{Time-Frequency Transform}
\label{app: Time-Frequency Transform}
The time-frequency (T-F) transform provides more detailed and comprehensive information across both time and frequency dimensions. In this work, the time-frequency representation is computed using the continuous wavelet transform (CWT), which is particularly suitable for non-stationary acoustic signal analysis because it captures localized signal characteristics at multiple scales. Formally, after applying the sliding-window operator $\mathcal{W}(\cdot)$, we obtain the subsequences $\{\mathbf{u}_{g,n}\}_{n=1}^{N_g}$ for recording $g$. For each subsequence $\mathbf{u}_{g,n}$, the CWT maps it into the time-frequency domain and is defined as:
\begin{equation}
\label{eq: CWT}
\mathcal{C}_{g,n}(a,b) = \frac{1}{\sqrt{|a|}} \sum\limits_{\ell=1}^{W_s} u_{g,n,\ell}\,\psi^*\left( \frac{\ell-b}{a} \right),
\end{equation}
where $\mathcal{C}_{g,n}(a,b)$ denotes the wavelet coefficient of the $n$-th window from recording $g$ at scale $a$ and translation $b$, $u_{g,n,\ell}=u_{g,(n-1)S+\ell}$ is the $\ell$-th sample in that window, $\psi(\cdot)$ is the mother wavelet, and $\psi^*(\cdot)$ represents its complex conjugate. The scale parameter $a$ controls the frequency resolution, while the translation parameter $b$ determines the temporal location of the wavelet. By varying $a$ and $b$, the CWT yields a multi-scale time-frequency representation for each acoustic subsequence. The essence of the CWT is to correlate the input signal with scaled and shifted versions of the mother wavelet, thereby revealing transient and non-stationary patterns across different frequency bands. In our method, the CWT plays an essential role in the preprocessing of the acoustic signal, where the coefficients $\mathcal{C}_{g,n}(a,b)$ of each subsequence $\mathbf{u}_{g,n}$ are converted into the RGB time-frequency image $I_{g,n}$ used in the main text. These images are subsequently used as the visual inputs of the diagnosis framework, together with the corresponding physical operating-condition vector $\mathbf{x}_g$.


\subsection{Experimental Settings and Reproducibility}
\label{app: Experimental Settings and Reproducibility}
\noindent\textbf{Computing environment.} The experiments are implemented in Python 3.10.19, with the deep-learning models using PyTorch 2.8.0, CUDA 12.9 and cuDNN 9.10.2 on an x86-64 Linux workstation. The workstation is equipped with an Intel Core i9-14900K processor with 32 logical processors and two NVIDIA GeForce RTX 5090 GPUs, each with approximately 32~GB of memory. Each deep-learning training job uses a single GPU, and four data-loading workers are used unless otherwise specified. The NVIDIA driver version is 595.71.05.

\noindent\textbf{Data partitioning and evaluation protocol.} The three datasets, Cavitation-Short, Cavitation-Long and Cavitation-Noise, are partitioned into training and held-out test sets at the original-recording level, using an approximately $80\%$/$20\%$ split. The exact numbers of recordings and the corresponding numbers of windows are given in Table \ref{tab: training and test sets}. Partitioning is completed before sliding-window segmentation and time-frequency transformation, so all windows from a recording $g$ remain in the same subset. A separate validation split is not used. POC-VLM is trained for a fixed schedule of 30 epochs without early stopping and evaluated on the predefined test set after training. The ablation results in Table \ref{tab:model_variants} are reported as the mean and standard deviation over three independent runs; the sensitivity and robustness results in Figures \ref{fig: AblationAnalysis} and \ref{fig: RobustnessAnalysis} are also averaged over three independent runs.


\noindent\textbf{Acoustic preprocessing and spectrogram generation.} Following Appendices \ref{app: Acoustic Signals Augmentation} and \ref{app: Time-Frequency Transform}, the waveform $\mathbf{u}_g$ is divided into windows $\mathbf{u}_{g,n}$. The default window duration is \SI{0.06}{s}, with an overlap ratio of 0.25. The window size and step size are $W_s=\operatorname{round}(0.06f_s)$ and $S=\operatorname{round}[W_s(1-0.25)]$, where $f_s$ is the effective sampling frequency and equals \SI{1562.5}{\kHz} in the default experiments. Each window is transformed using a real-valued Morlet wavelet and an FFT-based CWT implementation with sampling period $1/f_s$ and scales $a\in\{1,2,\ldots,512\}$. The complete pseudo-frequency range associated with these scales is retained. The wavelet coefficients $\mathcal{C}_{g,n}(a,b)$ in Eq. \ref{eq: CWT} are converted into a logarithmic amplitude representation:
\begin{equation}
A_{g,n}^{\mathrm{dB}}(a,b)=20\log_{10}\left(\left|\mathcal{C}_{g,n}(a,b)\right|+10^{-8}\right).
\end{equation}
For each window, the lower and upper colour limits are the 5th and 95th percentiles of $A_{g,n}^{\mathrm{dB}}$, with values outside this interval clipped to the corresponding limits. The result is rendered using the jet colour map over the complete window duration and pseudo-frequency range. Axes, tick labels and surrounding margins are removed, and the RGB spectrogram $I_{g,n}$ is saved as a square PNG image using a $4\times4$-inch canvas at 300~dpi. Window duration, overlap ratio and the number of CWT scales are varied individually in the sensitivity analysis in Figure \ref{fig: AblationAnalysis}; sampling frequency, noise level and cross-duration transfer are examined in Figure \ref{fig: RobustnessAnalysis}.

\noindent\textbf{Image preprocessing.} All spectrograms are loaded in RGB format. POC-VLM and the other image-based models use inputs of $224\times224$, except for the DenseNet baselines, which use $256\times256$. The training pipeline applies a horizontal flip, a vertical flip and a $180^\circ$ rotation, each deterministically, before resizing. These three operations together restore the original image orientation and therefore do not introduce stochastic geometric augmentation. At test time, the images are resized without flipping or rotation. Pixel intensities are converted from $[0,255]$ to $[0,1]$ and normalized separately for each RGB channel $r\in\{1,2,3\}$:
\begin{equation}
I_{g,n,r}^{\mathrm{norm}}=\frac{I_{g,n,r}-\mu_{\mathrm{img},r}}{\sigma_{\mathrm{img},r}},
\end{equation}
where $I_{g,n,r}$ denotes the rescaled intensities in channel $r$ of image $I_{g,n}$. The cavitation-image normalization constants are $\boldsymbol{\mu}_{\mathrm{img}}=[0.6317,0.5517,0.2756]$ and $\boldsymbol{\sigma}_{\mathrm{img}}=[0.2312,0.2368,0.2219]$, in RGB order. These statistics are obtained from training data and applied unchanged at test time. The channel index $r$ is distinct from the cavitation-class index $c$, and the image tensor is distinct from the physical operating-condition vector $\mathbf{x}_g$.

\noindent\textbf{POC-VLM configuration and optimization.} The same POC-VLM configuration is used for all three datasets. The pretrained CLIP ViT-B/16 visual and text encoders, $E_v$ and $E_t$, remain frozen. The global and local visual features have dimension 512, with $N_p=196$ local patches. The time-frequency-conditioned text adaptation module contains one cross-attention layer with eight heads and feature dimension 512. The residual scaling parameter $\boldsymbol{\gamma}$ is initialized to 0.1. The local matching branch uses $K_L=16$ patches, the normalized global and local matching weights $\alpha_G$ and $\alpha_L$ are initialized to 0.5, and $\tau$ is initialized to $1/0.07$. Candidate descriptions use the CLIP tokenizer with a context length of 77 tokens. Only the text adaptation and global-local matching modules are optimized using AdamW, with a batch size of 32 for 30 epochs. The weighted label-smoothed cross-entropy loss uses a smoothing factor of 0.02 and inverse-square-root class-frequency weights computed from the training set and normalized to a mean of one. The maximum gradient $L_2$ norm is 1.0. Further details of the loss and model configuration are given in Section \ref{subsec: Implementation Details}.

\noindent\textbf{Physical operating-condition processing.} The physical variables associated with recording $g$ are stored as 32-bit floating-point values in $\mathbf{x}_g$ and shared by all its windows. Image-only baselines use the spectrograms, physical-variable-driven baselines use the selected operating variables, and hybrid baselines use both modalities. In POC-VLM, the physical variables retain their original units when constructing $\mathcal{T}(c,\mathbf{x}_g)$. For the physical operating-condition prior, one labeled prototype is retained per training recording. The selected variables are standardized using the mean and population standard deviation computed exclusively from the training prototypes, yielding $\hat{\mathbf{x}}_g$ for distance calculations. The same statistics are applied to test recordings. This standardization is performed within the prior pathway, independently of the image normalization and the data loader. The prior uses $k=3$ nearest neighbours with inverse-distance weighting, and the final score uses $\lambda_{\text{POC}}=1$ and the probability floor $\delta=10^{-6}$ as defined in Eq. \ref{eq: final score}.

\noindent\textbf{Robustness experiments.} The experiments follow Section \ref{subsec: Generalization and Robustness Analysis} and Figure \ref{fig: RobustnessAnalysis}, covering sampling-frequency variation, additive noise and cross-duration transfer. Results for each setting are averaged over three independent runs. Sampling-frequency robustness on Cavitation-Short is evaluated at the original frequency $f_{s,0}=\SI{1562.5}{\kHz}$ and nominal target frequencies of 781.25, 390.625, 260.416, 195.312 and 48~\si{\kHz}, consistently with Figure \ref{fig: RobustnessAnalysis}(a). Each complete waveform $\mathbf{u}_g$ is resampled before sliding-window segmentation and CWT generation. Polyphase resampling incorporates low-pass anti-alias filtering. Integer decimation ratios are used when the target frequency is sufficiently close to an integer fraction of $f_{s,0}$. Otherwise, the target-to-original frequency ratio is represented by a rational upsampling and downsampling pair. The effective sampling frequency $f_s$ is calculated from the applied ratio and recorded for each generated sample. With $f_s$ expressed in hertz, the window size and step size are recalculated as $W_s=\operatorname{round}(0.06f_s)$ and $S=\operatorname{round}[W_s(1-0.25)]$, retaining the default duration of \SI{0.06}{s} and overlap ratio of 0.25. The real-valued Morlet wavelet, 512 scales and image-generation procedure are retained, with sampling period $1/f_s$ used in the CWT to generate $I_{g,n}$.

Noise robustness is evaluated at signal-to-noise ratios of $-5$, 0, 5, 10, 20 and 30~dB. For a clean acoustic signal $\mathbf{u}_g=[u_{g,1},\ldots,u_{g,L_g}]^{\mathrm T}$, the signal power is calculated as $P_{\mathrm{s}}=\frac{1}{L_g}\sum_{\ell=1}^{L_g}|u_{g,\ell}|^2$. For a specified signal-to-noise ratio $\mathrm{SNR}_{\mathrm{dB}}$, the target noise power and standard deviation are defined as $P_{\mathrm{n}}=\frac{P_{\mathrm{s}}}{10^{\mathrm{SNR}_{\mathrm{dB}}/10}}$ and $\sigma_{\mathrm{n}}=\sqrt{P_{\mathrm{n}}}$, respectively. Independent zero-mean Gaussian noise is then sampled as $\boldsymbol{\eta}_g\sim\mathcal{N}(\mathbf{0},\sigma_{\mathrm{n}}^2\mathbf{I}_{L_g})$, and the noisy signal is generated as $\widetilde{\mathbf{u}}_g=\mathbf{u}_g+\boldsymbol{\eta}_g$. Noise is added to the complete acoustic waveform before sliding-window segmentation and CWT generation. A separate deterministic random seed is constructed for each file--SNR pair as $s_{\mathrm{noise}}=\left[n_{\mathrm{file}}\times1000003+\operatorname{round}\bigl((\mathrm{SNR}_{\mathrm{dB}}+100)\times100\bigr)\right]\bmod 2^{32}$, where $n_{\mathrm{file}}$ denotes the numerical identifier of the original signal file. Consequently, different SNR levels use different noise realizations for the same signal, while repeated preprocessing with the same file and SNR reproduces the same noisy waveform. When the clean signal power is zero, the original signal is retained unchanged.

Cross-duration transfer in Figure \ref{fig: RobustnessAnalysis}(c) compares POC-VLM and PerceiverIO in both directions: training on Cavitation-Short and testing on Cavitation-Long, and training on Cavitation-Long and testing on Cavitation-Short. The original recordings last \SI{3}{s} and \SI{25}{s}, respectively, while the window duration remains \SI{0.06}{s}. The source training recordings provide the prototypes and standardization statistics for the physical prior of POC-VLM, which are then applied to the target recordings. For each robustness experiment, only the factor under investigation is varied; the remaining partitioning, preprocessing, architecture and optimization settings retain their default values.


\subsection{Evaluation Metrics}
\label{app: Evaluation Metrics}
The diagnosis task contains $C=4$ classes, indexed by $c\in\{1,\ldots,C\}$, consistently with the main text. For POC-VLM, the predicted class of window $(g,n)$ is $\hat{y}_{g,n}=\operatorname*{arg\,max}_{c}z_{g,n,c}^{\text{final}}$. Let $\mathrm{TP}_c$, $\mathrm{FP}_c$, $\mathrm{TN}_c$ and $\mathrm{FN}_c$ denote the true-positive, false-positive, true-negative and false-negative counts for class $c$ under a one-vs-rest formulation. The test support of class $c$ is $N_c^{\mathrm{test}}=\mathrm{TP}_c+\mathrm{FN}_c$, and the total number of evaluated test samples is $N_{\mathrm{test}}=\sum_{c=1}^{C}N_c^{\mathrm{test}}$. Counts are accumulated over the complete test set. The overall classification accuracy is:
\begin{equation}
\mathrm{Accuracy}=\frac{\sum_{c=1}^{C}\mathrm{TP}_c}{N_{\mathrm{test}}}.
\end{equation}

The class-specific precision, recall and F1-score are defined as:
\begin{equation}
\begin{aligned}
\mathrm{Precision}_c&=\frac{\mathrm{TP}_c}{\mathrm{TP}_c+\mathrm{FP}_c},\\
\mathrm{Recall}_c&=\frac{\mathrm{TP}_c}{\mathrm{TP}_c+\mathrm{FN}_c},\\
\mathrm{F1}_c&=\frac{2\,\mathrm{TP}_c}{2\,\mathrm{TP}_c+\mathrm{FP}_c+\mathrm{FN}_c}.
\end{aligned}
\end{equation}

Precision, recall and F1-score are calculated using macro averaging (\texttt{average="macro"}), assigning equal weight to each class regardless of its test support:
\begin{equation}
\begin{aligned}
\mathrm{Precision}_{\mathrm{macro}}&=\frac{1}{C}\sum_{c=1}^{C}\mathrm{Precision}_c,\\
\mathrm{Recall}_{\mathrm{macro}}&=\frac{1}{C}\sum_{c=1}^{C}\mathrm{Recall}_c,\\
\mathrm{F1}_{\mathrm{macro}}&=\frac{1}{C}\sum_{c=1}^{C}\mathrm{F1}_c.
\end{aligned}
\end{equation}
Macro F1 is the arithmetic mean of the class-specific F1-scores, rather than the harmonic mean of macro precision and macro recall. This convention gives the minority cavitation classes the same contribution as the majority classes. In particular, macro recall need not equal overall accuracy.
